# Supplementary material for: Budget-aware Query Tuning: An AutoML Perspective
Source: arXiv:2404.00137 source file (2024-03-29)
Supplement: Supplementary file 1 [file appendix.tex]

\section{Proposed Solution}

The main problem of the baseline solutions is that they treat the tuning of individual queries as \emph{independent} tasks.
In reality, these tuning tasks are often correlated, in the sense that the best cost units found for one query may also be the best ones for another query.
The reason is that many queries are similar in a workload (e.g., they may come from different parameterizations of the same query template).
We next propose new solutions by utilizing this similarity among queries.
\ww{Are there any properties that we can say about this solution?}

\ww{The goal is to tune important queries sufficiently.}

\subsection{A General Framework}

The general framework is the following:
\begin{itemize}
    \item Cluster the workload queries into $K$ groups based on their similarity. $K\geq 1$ is a number that depends on workload characteristics.
    \item (Cluster Selection) Select some query group/cluster $G$ with certain group/cluster selection policy.
    \item (Query Selection) Select some query $q\in G$ w.r.t. certain query selection policy.
    \item Tune $q$ for $L$ trials using an HPO searcher. $L$ is a number that depends on the current status of $q$.
    \item Let $\vec{u}_q$ be the best cost units found for $q$, and use $\vec{u}_q$ to check/validate all (or, a random sample of) other queries within the group $G$.
    \item For any other query $q'\in G$, mark $q'$ as tuned if $\vec{u}_q$ improves over $\vec{u}_0$, i.e., $t(q',\vec{u}_q) < t(q', \vec{u}_0)$ (or, based on some other improvement criterion).
    Otherwise, mark $q'$ as untuned.
    \item If all queries in $G$ are tuned, mark $G$ as tuned.
    \item Go to the cluster selection step and repeat.
\end{itemize}

\ww{This framework still looks too complicated to me.
For example, is it necessary to validate those queries with the best cost units? Why not just choose some representative queries from each cluster and use their cost units for other queries? It can then become a clustering problem.}

\ww{How can we break down the problem into smaller steps and then solve each step?}

\ww{Consider a simplest case where we have only one query template with many instances. How can we pick representative instances? We perhaps would cluster query instances with different parameter values but similar selectivity, because their execution costs should be similar (and therefore their best cost units should be similar, too). How can we formalize and generalize this idea?}

\subsection{Query Selection}

\textbf{How to select a query from a cluster?}
One approach is to use the UCB baseline here, which has been shown to perform the best among all the baselines that we have tested.
That is, we maintain the UCB score for each query in the cluster and always select the query with the largest UCB score.
Of course, this policy requires a ``warm up'' phase during which the selection of queries is close to random choice or round robin.

\subsection{Query Tuning Strategy}

\textbf{How many trials should we give to the selected query?}
One approach could be to just give it one trial, then this is reduced to the case of baseline approaches. The difference, of course, is the new query elimination process.

There is a trade-off here. If we allocate more trials to the selected query, then we can get more improvement on this query.
However, if this query is not \emph{pivotal}, i.e., its best cost units $\vec{u}$ is not the best or nearly the best for the other queries, then we end up wasting budget on tuning this query.

\textbf{Basic Question: How can we know that a query is pivotal without actually tuning all queries?}

\subsection{Query Elimination Strategy}

The strategy on query elimination (i.e., by marking a query as tuned) can have more variants.

\textbf{Basic Question: How can we know that a query has been sufficiently tuned so that additional improvement is low with further tuning?}

\subsection{Query Clustering}

\textbf{How to partition the entire workload into clusters/groups of queries?}
The criterion is correlated with the two basic questions for query tuning and elimination strategies, where we want to put queries with similar best cost units into the same cluster.

\ww{If two queries share many common subqueries, then they may also share similar best cost units, because the optimizer will return similar query plans for these common subqueries.}

\ww{We need to represent queries as feature vectors based on the above criteria and then cluster them based on some distance or similarity metric.}
